# Supplementary material for: AFCL: Analytic Federated Continual Learning for Spatio-Temporal Invariance of Non-IID Data
Source: arXiv:2505.12245 source file (2025-05-18)
Supplement: Supplementary file 1 [file X_suppl_old.tex]

\clearpage
\setcounter{page}{1}
% \maketitlesupplementary

% \onecolumn

\appendix


\begin{table*}[t]
    \centering
    \renewcommand{\arraystretch}{1.3}
    \caption{Description of important notations
    }
    \label{table-performance}
    % \small
        \begin{NiceTabular}{ l l }
        \toprule
        \textbf{Notations} & \textbf{Description} \\
        \midrule
        $\mathcal{X}_{k}$, $\mathcal{Y}_{k}$ & The $k$-th client's example set and label set, respectively.\\
        $\mathbf{F}_{k}$ & The $k$-th client's feature matrix.\\
        $\mathbf{\hat Y}_{k}$, $\mathbf{\check Y}_{k}$ & The $k$-th client's label matrices for known and unknown classes, respectively.\\
        $\mathbf{\hat W}_{k}$, $\mathbf{\check W}_{k}$ & The $k$-th client's regularized local weights for known and unknown classes, respectively.\\
        $\mathbf{R}_{k}$, $\mathbf{S}_{k}$ & The $k$-th client's regularized gram matrix and standard gram matrix, respectively. \\
        % $\mathbf{S}_{k}$ & The $k$-th client's standard gram matrix. \\
        $\mathbf{\widetilde R}_{k}$, $\mathbf{\widetilde S}_{k}$ & The sum of $\mathbf{R}_{k}$ and $\mathbf{S}_{k}$ for first $k$ clients, respectively. \\
        $\mathbf{G}_{k}$ & The global knowledge matrix up to the participation of the $k$-th client. \\
        $\mathbf{W}_{k}$ & The global weight up to the participation of the $k$-th client. \\
        
        \bottomrule
        \end{NiceTabular}
\end{table*}




\section{Theoretical Analysis} \label{appendix_A}


\noindent\textbf{Theorem 1:} Consider the optimization problem:
\begin{equation}
    \label{Proposition-1-1}
    \mathop{\arg\min}\limits_{\mathbf{W}} {\left\|\mathbf{Y} -\mathbf{F} \mathbf{W} \right\|}_F^2+\gamma{\left\| \mathbf{W} \right\|}_F^2,
\end{equation}
and the closed-form solution of this problem is:
\begin{equation}
    \label{Proposition-1-2}
    \mathbf{\hat W} = {({\mathbf{F}}^\top\mathbf{F}+\gamma\mathbf{I})}^{-1}{\mathbf{F}}^\top\mathbf{Y}.
\end{equation}

\noindent \textbf{\textit{Proof.}} According to \eqref{Proposition-2-1}, we can define the objective function as:
\begin{equation}
    \mathcal{L}(\mathbf{W})
    =\left\|\mathbf{Y}-\mathbf{F}\mathbf{W}\right\|_F^2 + \gamma \left\|W\right\|_F^2
    =\mathrm{Tr}\left[(\mathbf{Y}-\mathbf{F}\mathbf{W})^\top(\mathbf{Y}-\mathbf{F}\mathbf{W})\right] + \gamma \mathrm{Tr}( \mathbf{W}^\top \mathbf{W} ),
\end{equation}
which can be further expanded to:
\begin{equation}
    \mathcal{L}(\mathbf{W}) = \mathrm{Tr}(\mathbf{Y}^\top \mathbf{Y}) - 2\cdot\mathrm{Tr}(\mathbf{Y}^\top \mathbf{F} \mathbf{W}) + \mathrm{Tr}( \mathbf{W}^\top \mathbf{F}^\top \mathbf{F} \mathbf{W}) + \gamma \mathrm{Tr}(\mathbf{W}^\top \mathbf{W}).
\end{equation}
To find the minimizer $\mathbf{\hat W}$, we take the derivative of $\mathcal{L}(\mathbf{W})$, which can be calculated as follows:
\begin{equation}
\frac{ \partial \mathcal{L}(\mathbf{W}) }{\partial \mathbf{W}}
= -2\mathbf{F}^\top \mathbf{Y} + 2 \mathbf{F}^\top \mathbf{F} \mathbf{W} + 2 \gamma \mathbf{W}.
\end{equation}
By setting $\frac{ \partial \mathcal{L}(\mathbf{W}) }{\partial \mathbf{W}}=0$, we can obtain:
\begin{equation}
(\mathbf{F}^\top \mathbf{F} + \mathbf{I}) \mathbf{\hat W} = \mathbf{F}^\top \mathbf{Y}.
\end{equation}
Since $\mathbf{F}^\top \mathbf{F} + \mathbf{I}$ is positive-definite, we can obtain:
\begin{equation}
\mathbf{\hat W} =  (\mathbf{F}^\top \mathbf{F} + \mathbf{I})^{-1} \mathbf{F}^\top \mathbf{Y}.
\end{equation}

\hfill $\blacksquare$




\noindent\textbf{Inference 1:} The Global Knowledge Matrix $\mathbf{G}_{k}$ obtained using the complete dataset of the all $k$ clients $\mathcal{D}_{1:k}$ can be represented as:
\begin{equation}
\label{eq:appendix-A-inference-1-1}
\mathbf{G}_{k} = \begin{bmatrix} \sum_{i=1}^{k} ( \mathbf{F}_i^\top\mathbf{F}_i + \gamma \mathbf{I})\end{bmatrix}^{-1} \begin{bmatrix} \mathbf{F}_{1:k-1}^\top\mathbf{Y}_{1:k-1} + \mathbf{F}_k^\top\mathbf{\hat Y}_k  & \mathbf{F}_k^\top\mathbf{\check Y}_k   \end{bmatrix}.
\end{equation}


\noindent \textbf{\textit{Proof.}}
First, we denote the complete feature matrix and label matrix of all $k$ clients as $\mathbf{F}_{1:k}$ and $\mathbf{Y}_{1:k}$, respectively. Considering the presence of known and unknown classes in a class-incremental scenario, these matrices satisfy:
\begin{equation}
\label{eq:appendix-A-inference-1-2}
\mathbf{F}_{1:k} = \begin{bmatrix} \mathbf{F}_{1:k-1}\\ \mathbf{F}_{k} \end{bmatrix}, \quad \mathbf{Y}_{1:k} = \begin{bmatrix} \mathbf{Y}_{1:k-1} & \mathbf{0}\\ \mathbf{\hat Y}_{k} & \mathbf{\check Y}_{k} \end{bmatrix}.
\end{equation}

Therefore, we can obtain:
\begin{equation}
\label{eq:appendix-A-inference-1-3}
\begin{aligned}
    \mathbf{F}_{1:k}^\top \mathbf{F}_{1:k} &= \begin{bmatrix} \mathbf{F}_{1:k-1}^\top & \mathbf{F}_{k}^\top \end{bmatrix} \begin{bmatrix} \mathbf{F}_{1:k-1}\\ \mathbf{F}_{k} \end{bmatrix} \\
    &= \mathbf{F}_{1:k-1}^\top \mathbf{F}_{1:k-1} + \mathbf{F}_{k}^\top \mathbf{F}_{k} \\
    &= \sum\nolimits_{i=1}^k \mathbf{F}_{i}^\top \mathbf{F}_{i}.
\end{aligned}
\end{equation}
\begin{equation}
\label{eq:appendix-A-inference-1-4}
\begin{aligned}
    \mathbf{F}_{1:k}^\top \mathbf{Y}_{1:k} &= \begin{bmatrix} \mathbf{F}_{1:k-1}^\top & \mathbf{F}_{k}^\top \end{bmatrix} \begin{bmatrix} \mathbf{Y}_{1:k-1} & \mathbf{0}\\ \mathbf{\hat Y}_{k} & \mathbf{\check Y}_{k} \end{bmatrix} \\
    &= \begin{bmatrix} \mathbf{F}_{1:k-1}^\top \mathbf{Y}_{1:k-1} + \mathbf{F}_{k}^\top \mathbf{\hat Y}_{k} & \mathbf{F}_{k}^\top \mathbf{\check Y}_{k} \end{bmatrix} 
\end{aligned}
\end{equation}

By substituting \eqref{eq:appendix-A-inference-1-3} and \eqref{eq:appendix-A-inference-1-4} into \eqref{eq:Global Knowledge Matrix}, we can further derive:
\begin{equation}
\label{eq:appendix-A-inference-1-5}
\begin{aligned}
    \mathbf{G}_{k} &= \begin{bmatrix}
    \mathbf{F}_{1:k}^\top\mathbf{F}_{1:k} + \gamma \sum_{i=1}^k \mathbf{I} \end{bmatrix}^{-1} ( \mathbf{F}_{1:k}^\top\mathbf{Y}_{1:k} ) \\
    &= \begin{bmatrix}
    \sum_{i=1}^k \mathbf{F}_{i}^\top \mathbf{F}_{i} + \gamma \sum_{i=1}^k \mathbf{I} \end{bmatrix}^{-1} ( \mathbf{F}_{1:k}^\top\mathbf{Y}_{1:k} ) \\
    &= \begin{bmatrix} \sum_{i=1}^{k} ( \mathbf{F}_i^\top\mathbf{F}_i + \gamma \mathbf{I})\end{bmatrix}^{-1} \begin{bmatrix} \mathbf{F}_{1:k-1}^\top\mathbf{Y}_{1:k-1} + \mathbf{F}_k^\top\mathbf{\hat Y}_k  & \mathbf{F}_k^\top\mathbf{\check Y}_k   \end{bmatrix}.
\end{aligned}
\end{equation}

\hfill $\blacksquare$







\noindent\textbf{Theorem 2:} Let $\mathbf{G}_{k}$ and $\mathbf{G}_{k-1}$ represent the result of \eqref{eq:Global Knowledge Matrix} obtained using the complete dataset of the all $k$ clients $\mathcal{D}_{1:k}$ and the complete dataset of the first $k-1$ clients $\mathcal{D}_{1:k-1}$. It follows that:
\begin{equation}
\label{eq:appendix-A-theorem-2-1}
\mathbf{G}_{k} = \begin{bmatrix} \mathbf{A}_{k}  \mathbf{G}_{k-1} + \mathbf{B}_k  \mathbf{\hat W}_k & \mathbf{B}_k  \mathbf{\check W}_k \end{bmatrix},
\end{equation}
where
\begin{equation}
\label{eq:appendix-A-theorem-2-2}
\begin{cases}
\mathbf{A}_{k} = \mathbf{I} - (\mathbf{\tilde R}_{k-1})^{-1} \mathbf{R}_k (\mathbf{I} - (\mathbf{\tilde R}_{k})^{-1} \mathbf{R}_k),  \\
\mathbf{B}_{k} = \mathbf{I} - (\mathbf{R}_k)^{-1} \mathbf{\tilde R}_{k-1} (\mathbf{I} - (\mathbf{\tilde R}_{k})^{-1} \mathbf{\tilde R}_{k-1}), \\
\mathbf{\tilde R}_{k} = \sum_{i=1}^k \mathbf{R}_i, \quad
\mathbf{R}_i = \mathbf{F}_i^\top \mathbf{F}_i +\gamma\mathbf{I}.
\end{cases}
\end{equation}

\noindent \textbf{\textit{Proof.}}
According to \eqref{eq:Global Knowledge Matrix}, we can obtain that:
\begin{equation}
\label{eq:appendix-A-theorem-2-3}
\begin{aligned}
    \mathbf{G}_{k-1} 
    % &= [\sum_{i=1}^{k-1} ( \mathbf{F}_i^\top\mathbf{F}_i + \gamma \mathbf{I})]^{-1} \sum_{i=1}^{k-1} \mathbf{F}_i^\top\mathbf{Y}_i \\
    % &= (\sum_{i=1}^{k-1} \mathbf{R}_i)^{-1} \sum_{i=1}^{k-1} \mathbf{F}_i^\top\mathbf{Y}_i \\
    % &= (\mathbf{\tilde R}_{k-1})^{-1} \sum_{i=1}^{k-1} \mathbf{F}_i^\top\mathbf{Y}_i.\\
    &= \begin{bmatrix}
    \mathbf{F}_{1:k-1}^\top\mathbf{F}_{1:k-1} + \gamma \sum_{i=1}^{k-1} \mathbf{I} \end{bmatrix}^{-1} ( \mathbf{F}_{1:k-1}^\top\mathbf{Y}_{1:k-1} ) \\
    &= \begin{bmatrix}\sum_{i=1}^{k-1} ( \mathbf{F}_i^\top\mathbf{F}_i + \gamma \mathbf{I})\end{bmatrix}^{-1} ( \mathbf{F}_{1:k-1}^\top\mathbf{Y}_{1:k-1} ) \\
    &= (\mathbf{\tilde R}_{k-1})^{-1}( \mathbf{F}_{1:k-1}^\top\mathbf{Y}_{1:k-1} ) 
\end{aligned}
\end{equation}

Then, by substituting \eqref{eq:appendix-A-theorem-2-3} into $\mathbf{A}_{k}  \mathbf{G}_{k-1}$, we can obtain:
\begin{equation}
\label{eq:appendix-A-theorem-2-4}
  \begin{aligned}
\mathbf{A}_{k}  \mathbf{G}_{k-1} &= [ \mathbf{I} - (\mathbf{\tilde R}_{k-1})^{-1} \mathbf{R}_k (\mathbf{I} - (\mathbf{\tilde R}_{k})^{-1} \mathbf{R}_k) ] (\mathbf{\tilde R}_{k-1})^{-1} \mathbf{F}_{1:k-1}^\top\mathbf{Y}_{1:k-1} \\
&= [ \mathbf{I} - (\mathbf{\tilde R}_{k-1})^{-1} \mathbf{R}_k (\mathbf{I} - (\mathbf{R}_{k} + \mathbf{\tilde R}_{k-1})^{-1} \mathbf{R}_k) ] (\mathbf{\tilde R}_{k-1})^{-1} \mathbf{F}_{1:k-1}^\top\mathbf{Y}_{1:k-1} \\
&= [ \mathbf{I} - (\mathbf{\tilde R}_{k-1})^{-1}  (\mathbf{R}_k - \mathbf{R}_k(\mathbf{R}_{k} + \mathbf{\tilde R}_{k-1})^{-1} \mathbf{R}_k) ] (\mathbf{\tilde R}_{k-1})^{-1} \mathbf{F}_{1:k-1}^\top\mathbf{Y}_{1:k-1}\\
% &= [ (\mathbf{\tilde R}_{k-1})^{-1} - (\mathbf{\tilde R}_{k-1})^{-1} \mathbf{R}_k (\mathbf{I} + (\mathbf{\tilde R}_{k-1} + \mathbf{R}_{k})^{-1} \mathbf{R}_k) (\mathbf{\tilde R}_{k-1})^{-1}]  \sum\nolimits_{i=1}^{k-1}\mathbf{F}_i^\top\mathbf{Y}_i \\
% &= [ (\mathbf{\tilde R}_{k-1})^{-1} - (\mathbf{\tilde R}_{k-1})^{-1} \mathbf{R}_k (\mathbf{\tilde R}_{k-1})^{-1} - (\mathbf{\tilde R}_{k-1})^{-1} \mathbf{R}_k (\mathbf{\tilde R}_{k})^{-1} \mathbf{R}_k (\mathbf{\tilde R}_{k-1})^{-1}]  \sum\nolimits_{i=1}^{k-1}\mathbf{F}_i^\top\mathbf{Y}_i
  \end{aligned}
\end{equation}


According to the Woodbury Matrix Identity, for any matrices $\mathbf{A}\in\mathbb{R}^{n\times n}$, $\mathbf{B}\in\mathbb{R}^{n\times m}$, $\mathbf{E}\in\mathbb{R}^{m\times m}$, and $\mathbf{D}\in\mathbb{R}^{m\times n}$, the following equation holds consistently:
\begin{equation}
\label{eq:appendix-A-theorem-2-5}
(\mathbf{A}+\mathbf{B}\mathbf{E}\mathbf{D})^{-1}=\mathbf{A}^{-1}-\mathbf{A}^{-1}\mathbf{B}(\mathbf{E}^{-1}+\mathbf{D}\mathbf{A}^{-1}\mathbf{B})^{-1}\mathbf{D}\mathbf{A}^{-1}.
\end{equation}


Subsequently, based on \eqref{eq:appendix-A-theorem-2-5}, we substitute both $\mathbf{B}$ and $\mathbf{D}$ with $\mathbf{I}$. This adjustment allows us to derive:
\begin{equation}
\label{eq:appendix-A-theorem-2-6}
(\mathbf{A}+\mathbf{E})^{-1}=\mathbf{A}^{-1}-\mathbf{A}^{-1}(\mathbf{A}^{-1}+\mathbf{E}^{-1})^{-1}\mathbf{A}^{-1}
\end{equation}

Further, it can be obtained:
\begin{equation}
\label{eq:appendix-A-theorem-2-7}
\mathbf{A}^{-1}(\mathbf{A}^{-1}+\mathbf{E}^{-1})^{-1}\mathbf{A}^{-1} = \mathbf{A}^{-1} - (\mathbf{A}+\mathbf{E})^{-1}.
\end{equation}

By replacing $\mathbf{A}^{-1}$ and $\mathbf{E}^{-1}$ in \eqref{eq:appendix-A-theorem-2-7} with $\mathbf{R}_k$ and $\mathbf{\tilde R}_{k-1}$ respectively, yields:
\begin{equation}
\label{eq:appendix-A-theorem-2-8}
\mathbf{R}_k(\mathbf{R}_k+\mathbf{\tilde R}_{k-1})^{-1}\mathbf{R}_k = \mathbf{R}_k - ( (\mathbf{\tilde R}_{k-1})^{-1} + (\mathbf{R}_k)^{-1} )^{-1}
\end{equation}



Incorporating \eqref{eq:appendix-A-theorem-2-8} into \eqref{eq:appendix-A-theorem-2-4}, we can find:
\begin{equation}
\label{eq:appendix-A-theorem-2-9}
  \begin{aligned}
\mathbf{A}_{k}  \mathbf{G}_{k-1} &= [ \mathbf{I} - (\mathbf{\tilde R}_{k-1})^{-1}  (\mathbf{R}_k - \mathbf{R}_k(\mathbf{R}_{k} + \mathbf{\tilde R}_{k-1})^{-1} \mathbf{R}_k) ] (\mathbf{\tilde R}_{k-1})^{-1} \mathbf{F}_{1:k-1}^\top\mathbf{Y}_{1:k-1}\\
&= [ \mathbf{I} - (\mathbf{\tilde R}_{k-1})^{-1}  (\mathbf{R}_k - \mathbf{R}_k + ( (\mathbf{\tilde R}_{k-1})^{-1} + (\mathbf{R}_k)^{-1} )^{-1} )] (\mathbf{\tilde R}_{k-1})^{-1} \mathbf{F}_{1:k-1}^\top\mathbf{Y}_{1:k-1} \\
&= [ \mathbf{I} - (\mathbf{\tilde R}_{k-1})^{-1}  ( (\mathbf{\tilde R}_{k-1})^{-1} + (\mathbf{R}_k)^{-1} )^{-1} ] (\mathbf{\tilde R}_{k-1})^{-1} \mathbf{F}_{1:k-1}^\top\mathbf{Y}_{1:k-1}
  \end{aligned}
\end{equation}



\noindent Subsequently, replacing $\mathbf{A}$ and $\mathbf{E}$ in \eqref{eq:appendix-A-theorem-2-5} with $\mathbf{M}_i^\mathrm{r}$ and $\mathbf{M}_j^\mathrm{r}$ respectively, yields:
\begin{equation}
\label{eq:appendix-A-theorem-2-10}
(\mathbf{\tilde R}_{k-1})^{-1} ( (\mathbf{\tilde R}_{k-1})^{-1} + (\mathbf{R}_k)^{-1} )^{-1} (\mathbf{\tilde R}_{k-1})^{-1} = (\mathbf{\tilde R}_{k-1})^{-1} - (\mathbf{\tilde R}_{k-1}+\mathbf{R}_k)^{-1}
\end{equation}


Similarly, by incorporating \eqref{eq:appendix-A-theorem-2-10} into \eqref{eq:appendix-A-theorem-2-9}, we can obtain:
\begin{equation}
\label{eq:appendix-A-theorem-2-11}
  \begin{aligned}
\mathbf{A}_{k}  \mathbf{G}_{k-1} &= [ \mathbf{I} - (\mathbf{\tilde R}_{k-1})^{-1}  ( (\mathbf{\tilde R}_{k-1})^{-1} + (\mathbf{R}_k)^{-1} )^{-1} ] (\mathbf{\tilde R}_{k-1})^{-1} \mathbf{F}_{1:k-1}^\top\mathbf{Y}_{1:k-1} \\
&= [ (\mathbf{\tilde R}_{k-1})^{-1} - (\mathbf{\tilde R}_{k-1})^{-1}  ( (\mathbf{\tilde R}_{k-1})^{-1} + (\mathbf{R}_k)^{-1} )^{-1} (\mathbf{\tilde R}_{k-1})^{-1}]  \mathbf{F}_{1:k-1}^\top\mathbf{Y}_{1:k-1} \\
&= [ (\mathbf{\tilde R}_{k-1})^{-1} - (\mathbf{\tilde R}_{k-1})^{-1} + (\mathbf{\tilde R}_{k-1}+\mathbf{R}_k)^{-1}]  \mathbf{F}_{1:k-1}^\top\mathbf{Y}_{1:k-1} \\
&= (\mathbf{\tilde R}_{k})^{-1}  \mathbf{F}_{1:k-1}^\top\mathbf{Y}_{1:k-1} \\
  \end{aligned}
\end{equation}


Similarly, we can obtain:
\begin{equation}
\label{eq:appendix-A-theorem-2-12}
\mathbf{B}_k  \mathbf{\hat W}_k= (\mathbf{\tilde R}_{k})^{-1} \mathbf{F}_k^\top \mathbf{\hat Y}_j,
\end{equation}
\begin{equation}
\label{eq:appendix-A-theorem-2-13}
\mathbf{B}_k  \mathbf{\check W}_k = (\mathbf{\tilde R}_{k})^{-1} \mathbf{F}_k^\top \mathbf{\check Y}_j.
\end{equation}


By substituting \eqref{eq:appendix-A-theorem-2-11}, \eqref{eq:appendix-A-theorem-2-12}, and \eqref{eq:appendix-A-theorem-2-13} into \eqref{eq:appendix-A-theorem-2-1}, we can further derive:
\begin{equation}
\label{eq:appendix-A-theorem-2-14}
\begin{aligned}
    \mathbf{G}_{k} &= \begin{bmatrix} \mathbf{A}_{k}  \mathbf{G}_{k-1} + \mathbf{B}_k  \mathbf{\hat W}_k & \mathbf{B}_k  \mathbf{\check W}_k \end{bmatrix} \\
    &= \begin{bmatrix} (\mathbf{\tilde R}_{k})^{-1}  \mathbf{F}_{1:k-1}^\top\mathbf{Y}_{1:k-1} + (\mathbf{\tilde R}_{k})^{-1} \mathbf{F}_k^\top \mathbf{\hat Y}_j & (\mathbf{\tilde R}_{k})^{-1} \mathbf{F}_k^\top \mathbf{\check Y}_j \end{bmatrix} \\
    &= (\mathbf{\tilde R}_{k})^{-1} \begin{bmatrix} \mathbf{F}_{1:k-1}^\top\mathbf{Y}_{1:k-1} + \mathbf{F}_k^\top \mathbf{\hat Y}_j & \mathbf{F}_k^\top \mathbf{\check Y}_j \end{bmatrix} \\
    &=\begin{bmatrix} \sum_{i=1}^{k} ( \mathbf{F}_i^\top\mathbf{F}_i + \gamma \mathbf{I})\end{bmatrix}^{-1} \begin{bmatrix}\mathbf{F}_{1:k-1}^\top\mathbf{Y}_{1:k-1} + \mathbf{F}_k^\top\mathbf{\hat Y}_k  & \mathbf{F}_k^\top\mathbf{\check Y}_k   \end{bmatrix}.
\end{aligned}
\end{equation}

It is evident that the result obtained from \eqref{eq:appendix-A-theorem-2-1}, i.e., \eqref{eq:appendix-A-theorem-2-14}, is equivalent to the result of \eqref{eq:appendix-A-inference-1-1} in \textbf{Inference 1}, thereby confirming the correctness of our iterative update method for the Global Knowledge Matrix.

\hfill $\blacksquare$


\noindent\textbf{Theorem 3:} Let $\mathbf{W}_{k}$ and $\mathbf{G}_{k}$ represent the results of \eqref{Motivation-1} and \eqref{eq:Global Knowledge Matrix} obtained using the complete dataset of the all $k$ clients $\mathcal{D}_{1:k}$, while $\mathbf{\hat W}_{k}$ and $\mathbf{\check W}_{k}$ represent the results of \eqref{eq:client-3} and \eqref{eq:client-4} respectively using local datasets of the $k$-th client $\mathcal{D}_{k}$. It follows that:
\begin{equation}
\label{eq:appendix-A-theorem-3-1}
  \begin{aligned}
\mathbf{W}_k=[\mathbf{\tilde R}_{k} - (k-1)\gamma \mathbf{I}]^{-1} \mathbf{\tilde R}_{k} \mathbf{G}_{k},
\end{aligned}
\end{equation}
where
\begin{equation}
\label{eq:appendix-A-theorem-3-2}
\mathbf{\tilde R}_{k} = \sum_i^k \mathbf{R}_i, \quad
\mathbf{R}_i = \mathbf{F}_i^\top \mathbf{F}_i +\gamma\mathbf{I}.
\end{equation}

\noindent \textbf{\textit{Proof.}} According to \eqref{eq:Global Knowledge Matrix}, and \eqref{eq:appendix-A-theorem-3-2}, we can obtain that:
% \begin{equation}
%     \label{eq:appendix-A-theorem-3-3}
%     \begin{aligned}
%         \mathbf{W}_k &= {({\mathbf{F}}^\top_{1:k}  \mathbf{F}_{1:k}+\gamma\mathbf{I})}^{-1}({\mathbf{F}}^\top_{1:k} \mathbf{Y}_{1:k}) \\
%         &= ( \sum\nolimits_{i=1}^k {\mathbf{F}}^\top_k  \mathbf{F}_k + \gamma\mathbf{I}) ^{-1} ({\mathbf{F}}^\top_{1:k} \mathbf{Y}_{1:k}) \\
%         &= [ \mathbf{\tilde R}_k - (k-1)\gamma\mathbf{I} ] ^{-1} ({\mathbf{F}}^\top_{1:k} \mathbf{Y}_{1:k}),
%     \end{aligned}
% \end{equation}
\begin{equation}
    \label{eq:appendix-A-theorem-3-4}
    \begin{aligned}
    \mathbf{G}_k 
    &= \begin{bmatrix} \mathbf{F}_{1:k}^\top\mathbf{F}_{1:k} + \gamma \sum_{i=1}^k \mathbf{I} \end{bmatrix}^{-1} ( \mathbf{F}_{1:k}^\top\mathbf{Y}_{1:k} ) \\
    &= \begin{bmatrix} \sum\nolimits_{i=1}^k {\mathbf{F}}^\top_k {\mathbf{F}}_k + \gamma \sum_{i=1}^k \mathbf{I} \end{bmatrix}^{-1} ( \mathbf{F}_{1:k}^\top\mathbf{Y}_{1:k} ) \\
    &= \begin{bmatrix} \sum\nolimits_{i=1}^k ({\mathbf{F}}^\top_k {\mathbf{F}}_k + \gamma \mathbf{I}) \end{bmatrix}^{-1} ( \mathbf{F}_{1:k}^\top\mathbf{Y}_{1:k} ) \\
    &= ( \mathbf{\tilde R}_k ) ^{-1} ({\mathbf{F}}^\top_{1:k} \mathbf{Y}_{1:k}).
    \end{aligned}
\end{equation}

% Therefore, we can further obtain:
% \begin{equation}
%     \begin{aligned}
%         &[ \mathbf{\tilde R}_k - (k-1)\gamma\mathbf{I} ] \mathbf{\hat W}_k = \mathbf{\tilde R}_k \mathbf{G}_k \\
%         \Rightarrow &  \mathbf{W}_k = [ \mathbf{\tilde R}_k - (k-1)\gamma\mathbf{I} ]^{-1}\mathbf{\tilde R}_k \mathbf{G}_k.
%     \end{aligned}
% \end{equation}


By substituting \eqref{eq:appendix-A-theorem-3-4} into \eqref{eq:appendix-A-theorem-3-1}, we can further derive:
\begin{equation}
    \label{eq:appendix-A-theorem-3-5}
    \begin{aligned}
    \mathbf{W}_k
    &=[\mathbf{\tilde R}_{k} - (k-1)\gamma \mathbf{I}]^{-1} \mathbf{\tilde R}_{k} \mathbf{G}_{k} \\
    &=[\mathbf{\tilde R}_{k} - (k-1)\gamma \mathbf{I}]^{-1} \mathbf{\tilde R}_{k} ( \mathbf{\tilde R}_k ) ^{-1} ({\mathbf{F}}^\top_{1:k} \mathbf{Y}_{1:k}) \\
    &=[\mathbf{\tilde R}_{k} - (k-1)\gamma \mathbf{I}]^{-1} ({\mathbf{F}}^\top_{1:k} \mathbf{Y}_{1:k}) \\
    &=( \sum\nolimits_{i=1}^k {\mathbf{F}}^\top_k  \mathbf{F}_k + \gamma\mathbf{I}) ^{-1} ({\mathbf{F}}^\top_{1:k} \mathbf{Y}_{1:k}) \\
    &={({\mathbf{F}}^\top_{1:k}  \mathbf{F}_{1:k}+\gamma\mathbf{I})}^{-1}({\mathbf{F}}^\top_{1:k} \mathbf{Y}_{1:k})
    \end{aligned}
\end{equation}

It is evident that the result derived from \eqref{eq:server-5}, i.e., \eqref{eq:appendix-A-theorem-3-1}, is equivalent to the centralized result of \eqref{Motivation-2} obtained using the complete dataset of all $k$ clients $\mathcal{D}_{1:k}$, thereby validating the correctness of our scheme.

\hfill $\blacksquare$


In summary, the global model $\mathbf{W}_k$ obtained by our AFCL scheme through federated learning is fully equivalent to the result derived from centralized training using the complete dataset.

























\clearpage


% 前一版的证明：

\noindent\textbf{Proposition 1:} Consider the optimization problem:
\begin{equation}
    \label{Proposition-1-1}
    \mathop{\arg\min}\limits_{\mathbf{W}} {\left\|\mathbf{Y} -\mathbf{X} \mathbf{W} \right\|}_F^2,
\end{equation}
and the closed-form solution of this problem is:
\begin{equation}
    \label{Proposition-1-2}
    \mathbf{\hat W} = \mathbf{X}^{\dagger} \mathbf{ Y}.
\end{equation}

\noindent \textbf{\textit{Proof.}}
Let us define its objective function as:
\begin{equation}
    \mathcal{L}(\mathbf{W})=\left\|\mathbf{Y}-\mathbf{X}\mathbf{W}\right\|_F^2=\mathrm{Tr}\left[(\mathbf{Y}-\mathbf{X}\mathbf{W})^\top(\mathbf{Y}-\mathbf{X}\mathbf{W})\right],
\end{equation}
where $\mathrm{Tr}( \cdot )$ denotes the trace of a matrix. To find the minimizer $\mathbf{\hat W}$, we take the derivative of $\mathcal{L}(\mathbf{W})$, which can be calculated as follows:
\begin{equation}
\frac{ \partial \mathcal{L}(\mathbf{W}) }{\partial \mathbf{W}}
=-2\mathbf{X}^\top (\mathbf{Y} -  \mathbf{X}\mathbf{W} )
\end{equation}

\noindent By setting $\frac{ \partial \mathcal{L}(\mathbf{W}) }{\partial \mathbf{W}}=0$ we can obtain:
\begin{equation}
\mathbf{X}^\top \mathbf{X} \mathbf{\hat W} = \mathbf{X}^\top \mathbf{Y}.
\end{equation}

\noindent Since $\mathbf{X}^\top \mathbf{X}$ may be singular or $\mathbf{X}$ may be rank-deficient, we utilize the MP inverse to obtain the least-squares solution:
\begin{equation}
    \mathbf{\hat W} = \mathbf{X}^{\dagger} \mathbf{ Y}.
\end{equation}

\hfill $\blacksquare$


\noindent\textbf{Proposition 2:} Consider the optimization problem:
\begin{equation}
    \label{Proposition-2-1}
    \mathop{\arg\min}\limits_{\mathbf{W}} {\left\|\mathbf{Y} -\mathbf{X} \mathbf{W} \right\|}_F^2+\gamma{\left\| \mathbf{W} \right\|}_F^2,
\end{equation}
and the closed-form solution of this problem is:
\begin{equation}
    \label{Proposition-2-2}
    \mathbf{\hat W} = {({\mathbf{X}}^\top\mathbf{X}+\gamma\mathbf{I})}^{-1}{\mathbf{X}}^\top\mathbf{Y}.
\end{equation}

\noindent \textbf{\textit{Proof.}} According to \eqref{Proposition-2-1}, we can define the objective function as:
\begin{equation}
    \mathcal{L}(\mathbf{W})
    =\left\|\mathbf{Y}-\mathbf{X}\mathbf{W}\right\|_F^2 + \gamma \left\|W\right\|_F^2
    =\mathrm{Tr}\left[(\mathbf{Y}-\mathbf{X}\mathbf{W})^\top(\mathbf{Y}-\mathbf{X}\mathbf{W})\right] + \gamma \mathrm{Tr}( \mathbf{W}^\top \mathbf{W} ),
\end{equation}
which can be further expanded to:
\begin{equation}
    \mathcal{L}(\mathbf{W}) = \mathrm{Tr}(\mathbf{Y}^\top \mathbf{Y}) - 2\cdot\mathrm{Tr}(\mathbf{Y}^\top \mathbf{X} \mathbf{W}) + \mathrm{Tr}( \mathbf{W}^\top \mathbf{X}^\top \mathbf{X} \mathbf{W}) + \gamma \mathrm{Tr}(\mathbf{W}^\top \mathbf{W}).
\end{equation}
To find the minimizer $\mathbf{\hat W}$, we take the derivative of $\mathcal{L}(\mathbf{W})$, which can be calculated as follows:
\begin{equation}
\frac{ \partial \mathcal{L}(\mathbf{W}) }{\partial \mathbf{W}}
= -2\mathbf{X}^\top \mathbf{Y} + 2 \mathbf{X}^\top \mathbf{X} \mathbf{W} + 2 \gamma \mathbf{W}.
\end{equation}
By setting $\frac{ \partial \mathcal{L}(\mathbf{W}) }{\partial \mathbf{W}}=0$, we can obtain:
\begin{equation}
(\mathbf{X}^\top \mathbf{X} + \mathbf{I}) \mathbf{\hat W} = \mathbf{X}^\top \mathbf{Y}.
\end{equation}
Since $\mathbf{X}^\top \mathbf{X} + \mathbf{I}$ is positive-definite, we can obtain:
\begin{equation}
\mathbf{\hat W} =  (\mathbf{X}^\top \mathbf{X} + \mathbf{I})^{-1} \mathbf{X}^\top \mathbf{Y}.
\end{equation}

\hfill $\blacksquare$

\clearpage











To illustrate this process clearly, we first consider a scenario with two clients, denoted as client $i$ and client $j$, where the complete dataset is $\mathbf{X} = \begin{bmatrix} \mathbf{X}_i \\ \mathbf{X}_j\end{bmatrix}$ and $\mathbf{Y} = \begin{bmatrix} \mathbf{Y}_i & \textbf{0} \\ \mathbf{\bar Y}_j & \mathbf{\tilde Y}_j  \end{bmatrix}$. 

% For the client $i$, the model weights can be computed as:
% \begin{small} 
% \begin{equation*}
%    \mathbf{W}_i^\mathrm{r} = (\mathbf{M}_i^\mathrm{r})^{-1}\mathbf{X}_i^\top\mathbf{ Y}_i,
%    \mathbf{M}_i^\mathrm{r} = \mathbf{X}_i^\top \mathbf{X}_i +\gamma\mathbf{I},
% \end{equation*}
% \end{small} 

% For the client $j$, the model weights can be computed as:
% \begin{small} 
% \begin{equation*}
%    \hat{\mathbf{W}}_j^\mathrm{r} =(\mathbf{M}_j^\mathrm{r})^{-1}\mathbf{X}_k^\top\mathbf{\bar Y}_j, 
%    \check{\mathbf{W}}_j^\mathrm{r} =(\mathbf{M}_j^\mathrm{r})^{-1}\mathbf{X}_k^\top\mathbf{\tilde Y}_j,
%    \mathbf{M}_j^\mathrm{r} = \mathbf{X}_j^\top \mathbf{X}_j +\gamma\mathbf{I}. 
% \end{equation*}
% \end{small} 



% Moreover, we can further extend the model aggregation from two clients to multiple clients.




\noindent \textbf{Lemma 1:} For $\mathbf{X}=\begin{bmatrix}\mathbf{X}_i\\\mathbf{X}_j\end{bmatrix}$ , composed of two matrices $\mathbf{X}_{i}$ and $\mathbf{X}_{j}$ both satisfying column full rank, its MP inverse $\mathbf{X}_{k}^{\dagger}$ adheres to the following partition:
\begin{equation}
\label{eq:Lema_1}
  \mathbf{X}^{\dagger}=\begin{bmatrix}\bar{\mathbf{U}}&\bar{\mathbf{V}}\end{bmatrix},
\end{equation}
where
\begin{equation}
\label{eq:Lema_2}
\begin{cases}
\mathbf{\bar{U}} = \mathbf{X}_i^\dagger - \mathbf{M}_i^{-1} \mathbf{M}_j \mathbf{X}_i^\dagger - \mathbf{M}_i^{-1} \mathbf{M}_j (\mathbf{M}_i + \mathbf{M}_j)^{-1} \mathbf{M}_j \mathbf{X}_i^\dagger, \\
\mathbf{\bar{V}} = \mathbf{X}_j^\dagger - \mathbf{M}_j^{-1} \mathbf{M}_i \mathbf{X}_j^\dagger - \mathbf{M}_j^{-1} \mathbf{M}_i (\mathbf{M}_i + \mathbf{M}_j)^{-1} \mathbf{M}_i \mathbf{X}_j^\dagger, \\
\mathbf{M}_i = \mathbf{X}_i^\top \mathbf{X}_i, \quad \quad \mathbf{M}_j = \mathbf{X}_j^\top \mathbf{X}_j.
\end{cases}
\end{equation}



\noindent \textbf{\textit{Proof.}} Existing research on MP inverse partitioning \cite{AL_7} has demonstrated that the MP inverse of any matrix $\mathbf{A}=[\mathbf{U}\quad\mathbf{V}]$ can be expressed as follows:


\begin{equation}
\label{eq:appendix1_1}
  \mathbf{A}^\dagger = [\mathbf{U}\quad \mathbf{V}]^\dagger
     = \begin{bmatrix}\mathbf{U}^\dagger-\mathbf{U}^\dagger \mathbf{V}\mathbf{M}^\dagger-\mathbf{U}^\dagger \mathbf{V}(\mathbf{I}-\mathbf{M}^\dagger \mathbf{M})\mathbf{K}\mathbf{V}^*\mathbf{U}^\dagger*\mathbf{U}^\dagger(\mathbf{I}-\mathbf{V}\mathbf{M}^\dagger)\\\mathbf{V}^\dagger-\mathbf{V}^\dagger \mathbf{U}\tilde{\mathbf{M}}^\dagger-\mathbf{V}^\dagger \mathbf{U}(\mathbf{I}-\tilde{\mathbf{M}}^\dagger\tilde{\mathbf{M}})\tilde{\mathbf{K}}\mathbf{U}^*\mathbf{V}^\dagger*\mathbf{V}^\dagger(\mathbf{I}-\mathbf{U}\tilde{\mathbf{M}}^\dagger)\end{bmatrix},
\end{equation}
where

\begin{equation}
\label{eq:appendix1_2}
\begin{cases}
\mathbf{M}=(\mathbf{I}-\mathbf{U}\mathbf{U}^\dagger)\mathbf{V}\\
\mathbf{\tilde{M}}=(\mathbf{I}-\mathbf{V}\mathbf{V}^\dagger)\mathbf{U}
\end{cases},\quad
\begin{cases}
\mathbf{K}=\begin{bmatrix}
\mathbf{I}+(\mathbf{I}-\mathbf{M}^\dagger\mathbf{M})\mathbf{V}^*\mathbf{U}^\dagger*\mathbf{U}^\dagger\mathbf{V}(\mathbf{I}-\mathbf{M}^\dagger\mathbf{M})
\end{bmatrix}^{-1}\\
\mathbf{\tilde{K}}=\begin{bmatrix}
\mathbf{I}+(\mathbf{I}-\mathbf{M}^\dagger\mathbf{M})\mathbf{U}^*\mathbf{V}^\dagger*\mathbf{V}^\dagger\mathbf{U}(\mathbf{I}-\mathbf{M}^\dagger\mathbf{M})
\end{bmatrix}^{-1}
\end{cases}.
\end{equation}


\noindent Furthermore, by substituting $\mathbf{X}_i^\top $ for $\mathbf{U}$ and $\mathbf{X}_j^\top $ for $\mathbf{V}$, (\ref{eq:appendix1_1}) and (\ref{eq:appendix1_2}) can be transformed as follows:

\begin{equation}
\label{eq:appendix1_3}
  \mathbf{X}^{\dagger}=\begin{bmatrix}\mathbf{X}_{i}\\\mathbf{X}_{j}\end{bmatrix}^{\dagger}=\begin{bmatrix}\mathbf{X}_{i}^{\dagger\top}-\mathbf{X}_{i}^{\dagger\top}\mathbf{X}_{j}^{\top}\mathbf{M}^{\dagger}-\mathbf{X}_{i}^{\dagger\top}\mathbf{X}_{j}^{\top}(\mathbf{I}-\mathbf{M}^{\dagger}\mathbf{M})\mathbf{K}\mathbf{X}_{j}\mathbf{X}_{i}^{\dagger}\mathbf{X}_{i}^{\dagger\top}(\mathbf{I}-\mathbf{X}_{j}^{\top}\mathbf{M}^{\dagger}),\\
\mathbf{X}_{j}^{\dagger\top}-\mathbf{X}_{j}^{\dagger\top}\mathbf{X}_{i}^{\top}\tilde{\mathbf{M}}^{\dagger}-\mathbf{X}_{j}^{\dagger\top}\mathbf{X}_{i}^{\top}(\mathbf{I}-\tilde{\mathbf{M}}^{\dagger}\tilde{\mathbf{M}})\tilde{\mathbf{K}}\mathbf{X}_{i}\mathbf{X}_{j}^{\dagger}\mathbf{X}_{j}^{\dagger\top}(\mathbf{I}-\mathbf{X}_{i}^{\top}\tilde{\mathbf{M}}^{\dagger})\end{bmatrix}^{\top},
\end{equation}
where

\begin{equation}
\label{eq:appendix1_4}
  \begin{cases}
\mathbf{M}=(\mathbf{I}-\mathbf{X}_i^\top\mathbf{X}_i^{\dagger\top})\mathbf{X}_j^\top \\
\mathbf{\tilde{M}}=(\mathbf{I}-\mathbf{X}_j^\top\mathbf{X}_j^{\dagger\top})\mathbf{X}_i^\top
\end{cases},\quad
\begin{cases}
\mathbf{K}=\begin{bmatrix}
\mathbf{I}+(\mathbf{I}-\mathbf{M}^\dagger\mathbf{M})\mathbf{X}_j\mathbf{X}_i^\dagger\mathbf{X}_i^\dagger\top\mathbf{X}_j^\top(\mathbf{I}-\mathbf{M}^\dagger\mathbf{M})
\end{bmatrix}^{-1} \\
\mathbf{\tilde{K}}=\begin{bmatrix}
\mathbf{I}+(\mathbf{I}-\mathbf{M}^\dagger\mathbf{M})\mathbf{X}_i\mathbf{X}_j^\dagger\mathbf{X}_j^\dagger\top\mathbf{X}_i^\top(\mathbf{I}-\mathbf{M}^\dagger\mathbf{M})
\end{bmatrix}^{-1}
\end{cases}.
\end{equation}

\noindent Given that both $\mathbf{X}_i$ and $\mathbf{X}_j$ possess column full rank, their MP inverses can be computed as:

\begin{equation}
\label{eq:appendix1_5}
\mathbf{X}_i^\dagger=(\mathbf{X}_i^\top\mathbf{X}_i)^{-1}\mathbf{X}_i^\top,
\quad\mathbf{X}_j^\dagger=(\mathbf{X}_j^\top\mathbf{X}_j)^{-1}\mathbf{X}_j^\top.
\end{equation}


\noindent Substituting (\ref{eq:appendix1_5}) into (\ref{eq:appendix1_4}) yields that $\mathbf{M}$ and $\mathbf{\tilde{M}}$ can be computed as:
\begin{equation}
\label{eq:appendix1_6}
  \begin{cases}
\mathbf{M}=(\mathbf{I}-\mathbf{X}_i^\top\mathbf{X}_i^{\dagger\top})\mathbf{X}_j^\top = (\mathbf{I}-\mathbf{X}_i^\top\mathbf{X}_i(\mathbf{X}_i^\top\mathbf{X}_i)^{-1})\mathbf{X}_j^\top=\mathbf{0} \\
\mathbf{\tilde{M}}=(\mathbf{I}-\mathbf{X}_j^\top\mathbf{X}_j^{\dagger\top})\mathbf{X}_i^\top = (\mathbf{I}-\mathbf{X}_j^\top\mathbf{X}_j(\mathbf{X}_j^\top\mathbf{X}_j)^{-1})\mathbf{X}_i^\top=\mathbf{0}
\end{cases}
\end{equation}


\noindent Furthermore, $\mathbf{K}$ and $\mathbf{\tilde{K}}$ can be calculated as:
\begin{equation}
\label{eq:appendix1_7}
\begin{cases}
\mathbf{K}=\begin{bmatrix}
\mathbf{I}+(\mathbf{I}-\mathbf{M}^\dagger\mathbf{M})\mathbf{X}_j\mathbf{X}_i^\dagger\mathbf{X}_i^\dagger\top\mathbf{X}_j^\top(\mathbf{I}-\mathbf{M}^\dagger\mathbf{M})
\end{bmatrix}^{-1}=(\mathbf{I}+\mathbf{X}_{j}\mathbf{X}_{i}^{\dagger}\mathbf{X}_{i}^{\dagger\top}\mathbf{X}_{j}^{\top})^{-1}\\
\mathbf{\tilde{K}}=\begin{bmatrix}
\mathbf{I}+(\mathbf{I}-\mathbf{M}^\dagger\mathbf{M})\mathbf{X}_i\mathbf{X}_j^\dagger\mathbf{X}_j^\dagger\top\mathbf{X}_i^\top(\mathbf{I}-\mathbf{M}^\dagger\mathbf{M})
\end{bmatrix}^{-1}=(\mathbf{I}+\mathbf{X}_{i}\mathbf{X}_{j}^{\dagger}\mathbf{X}_{j}^{\dagger\top}\mathbf{X}_{i}^{\top})^{-1}
\end{cases}
\end{equation}

\noindent Meanwhile, (\ref{eq:appendix1_3}) can also be reduced to:
\begin{equation}
\label{eq:appendix1_8}
\mathbf{X}^\dagger=\begin{bmatrix}
\mathbf{X}_i^{\dagger\top}-\mathbf{X}_i^{\dagger\top}\mathbf{X}_j^{\top}\mathbf{K}\mathbf{X}_j\mathbf{X}_i^{\dagger}\mathbf{X}_i^{\dagger\top} \\
\mathbf{X}_j^{\dagger\top}-\mathbf{X}_j^{\dagger\top}\mathbf{X}_i^{\top}\mathbf{K}\mathbf{X}_i\mathbf{X}_j^{\dagger}\mathbf{X}_j^{\dagger\top}
\end{bmatrix}^\top
\end{equation}


\noindent Subsequently, applying the Woodbury Matrix Identity reveals that for conformable matrices $\mathbf{A}\in\mathbb{R}^{n\times n}$, $\mathbf{B}\in\mathbb{R}^{n\times m}$, $\mathbf{E}\in\mathbb{R}^{m\times m}$, and $\mathbf{D}\in\mathbb{R}^{m\times n}$, (\ref{eq:appendix1_8}) consistently holds.
\begin{equation}
\label{eq:appendix1_9}
(\mathbf{A}+\mathbf{B}\mathbf{E}\mathbf{D})^{-1}=\mathbf{A}^{-1}-\mathbf{A}^{-1}\mathbf{B}(\mathbf{E}^{-1}+\mathbf{D}\mathbf{A}^{-1}\mathbf{B})^{-1}\mathbf{D}\mathbf{A}^{-1}.
\end{equation}

\noindent By substituting $\mathbf{A}$ with $\mathbf{I}$, $\mathbf{I}$ with $\mathbf{X}_j$, $\mathbf{E}$ with $\mathbf{X}_i^\dagger \mathbf{X}_i^{\dagger\top}$, and $\mathbf{D}$ with $\mathbf{X}_j^\top$ in (\ref{eq:appendix1_9}), we derive the following result:
\begin{equation}
\label{eq:appendix1_10}
\mathbf{K}=\mathbf{I}-\mathbf{X}_j(\mathbf{X}_i^\top\mathbf{X}_i+\mathbf{X}_j^\top\mathbf{X}_j)^{-1}\mathbf{X}_j^\top.
\end{equation}

\noindent Similarly, we can obtain 
\begin{equation}
\label{eq:appendix1_11}
\mathbf{\tilde{K}}=\mathbf{I}-\mathbf{X}_i(\mathbf{X}_i^\top \mathbf{X}_i+\mathbf{X}_j^\top \mathbf{X}_j)^{-1}\mathbf{X}_i^\top.
\end{equation}

\noindent Let $X^\dagger=\begin{bmatrix}\bar{U}&\bar{V}\end{bmatrix}$, we have
\begin{equation}
\label{eq:appendix1_12}
\begin{cases}
\mathbf{\bar{U}}=(\mathbf{X}_i^{\dagger\top}-\mathbf{X}_i^{\dagger\top}\mathbf{X}_j^{\top}\mathbf{K}\mathbf{X}_j\mathbf{X}_i^{\dagger}\mathbf{X}_i^{\dagger\top})^{\top}=\mathbf{X}_i^{\dagger}-\mathbf{X}_i^{\dagger}\mathbf{X}_i^{\dagger\top}\mathbf{X}_j^{\top}\mathbf{K}^{\top}\mathbf{X}_j\mathbf{X}_i^{\dagger} \\
\mathbf{\bar{V}}=\left(\mathbf{X}_j^{\dagger\top}-\mathbf{X}_j^{\dagger\top}\mathbf{X}_i^{\top}\mathbf{\tilde{K}}\mathbf{X}_i\mathbf{X}_j^{\dagger}\mathbf{X}_j^{\dagger\top}\right)^{\top}=\mathbf{X}_j^{\dagger}-\mathbf{X}_j^{\dagger}\mathbf{X}_j^{\dagger\top}\mathbf{X}_i^{\top}\mathbf{\tilde{K}}^{\top}\mathbf{X}_i\mathbf{X}_j^{\dagger}
\end{cases}
\end{equation}

\noindent By substituting $\mathbf{K}$ and $\mathbf{\tilde{K}}$ from (\ref{eq:appendix1_10}) and (\ref{eq:appendix1_11}) into (\ref{eq:appendix1_12}), we can obtained:
\begin{equation}
\label{eq:appendix1_13}
\begin{cases}
\mathbf{\bar{U}}=\mathbf{X}_i^\dagger-\mathbf{X}_i^\dagger\mathbf{X}_i^{\dagger\top}\mathbf{X}_j^\top\left(\mathbf{I}-\mathbf{X}_j(\mathbf{X}_i^\top\mathbf{X}_i+\mathbf{X}_j^\top\mathbf{X}_j)^{-1}\mathbf{X}_j^\top\right)^\top\mathbf{X}_j\mathbf{X}_i^\dagger \\
\mathbf{\bar{V}}=\mathbf{X}_j^\dagger-\mathbf{X}_j^\dagger\mathbf{X}_j^\dagger\top\mathbf{X}_i^\top\left(\mathbf{I}-\mathbf{X}_i(\mathbf{X}_i^\top\mathbf{X}_i+\mathbf{X}_j^\top\mathbf{X}_j)^{-1}\mathbf{X}_i^\top\right)^\top\mathbf{X}_i\mathbf{X}_j^\dagger
\end{cases}
\end{equation}

\noindent That is,
\begin{equation}
\label{eq:appendix1_14}
\begin{cases}
\mathbf{\bar{U}} = \mathbf{X}_i^\dagger - \mathbf{X}_i^\dagger \mathbf{X}_i^{\dagger\top} \mathbf{X}_j^\top \mathbf{X}_j \mathbf{X}_i^\dagger - \mathbf{X}_i^\dagger \mathbf{X}_i^\dagger \mathbf{X}_j^\top \mathbf{X}_j (\mathbf{X}_i^\top \mathbf{X}_i + \mathbf{X}_j^\top \mathbf{X}_j)^{-1} \mathbf{X}_j^\top \mathbf{X}_j \mathbf{X}_i^\dagger \\
\mathbf{\bar{V}} = \mathbf{X}_j^\dagger - \mathbf{X}_j^\dagger \mathbf{X}_j^{\dagger\top} \mathbf{X}_i^\top \mathbf{X}_i \mathbf{X}_j^\dagger - \mathbf{X}_j^\dagger \mathbf{X}_j^\dagger \mathbf{X}_i^\top \mathbf{X}_i (\mathbf{X}_i^\top \mathbf{X}_i + \mathbf{X}_j^\top \mathbf{X}_j)^{-1} \mathbf{X}_i^\top \mathbf{X}_i \mathbf{X}_j^\dagger
\end{cases}
\end{equation}

\noindent We denote
\begin{equation}
\label{eq:appendix1_15}
\left.\left\{\begin{matrix}
\mathbf{M}_i=\mathbf{X}_i^\top \mathbf{X}_i \\
\mathbf{M}_j=\mathbf{X}_j^\top \mathbf{X}_j
\end{matrix}\right.\right., \left\{\begin{matrix}
\mathbf{R}_i=\mathbf{M}_i^{-1} \\
\mathbf{R}_j=\mathbf{M}_j^{-1}
\end{matrix}.\right.
\end{equation}

\noindent Consequently, (\ref{eq:appendix1_14}) can be rewritten as:
\begin{equation}
\label{eq:appendix1_16}
\begin{cases}
\mathbf{\bar{U}} = \left[\mathbf{I} - \mathbf{R}_i \mathbf{M}_j - \mathbf{R}_i \mathbf{M}_j (\mathbf{M}_i + \mathbf{M}_j)^{-1} \mathbf{M}_j \right] \mathbf{X}_i^\dagger \\
\mathbf{\bar{V}} = \left[\mathbf{I} - \mathbf{R}_j \mathbf{M}_i - \mathbf{R}_j \mathbf{M}_i (\mathbf{M}_i + \mathbf{M}_j)^{-1} \mathbf{M}_i \right] \mathbf{X}_j^\dagger
\end{cases}
\end{equation}

\noindent Thus, 
\begin{equation}
\label{eq:appendix1_17}
\mathbf{X}^\dagger = \begin{bmatrix} \mathbf{X}_i \\ \mathbf{X}_j \end{bmatrix}^\dagger = 
\begin{bmatrix} \mathbf{\bar{U}} & \mathbf{\bar{V}} \end{bmatrix}
\end{equation}

\noindent Based on (\ref{eq:appendix1_15}), (\ref{eq:appendix1_16}), and (\ref{eq:appendix1_17}), the proof is completed. 

\hfill $\blacksquare$


% \clearpage
%%%%%%%%%%%%%%%%%%%%%%%%%%%%%%%%%%%%%%%%%%%%%%%%%%%%%%%%%%%%%%%%




\noindent \textbf{Proposition 3.} Let ${\mathbf{W}} = \mathbf{X}^\dagger \mathbf{Y}$, $\mathbf{X} = \begin{bmatrix} \mathbf{X}_i \\ \mathbf{X}_j\end{bmatrix}$ and $\mathbf{Y} = \begin{bmatrix} \mathbf{Y}_i & \textbf{0} \\ \mathbf{\bar Y}_j & \mathbf{\tilde Y}_j  \end{bmatrix}$, where $\mathbf{X}_i$ and $\mathbf{X}_j$ both have full column ranks. Meanwhile, let $\mathbf{W}_i = \mathbf{X}_i^\dagger \mathbf{Y}_i$, $\mathbf{\hat{W}}_j = \mathbf{X}_j^\dagger \mathbf{\bar Y}_j$ and $\mathbf{\check{W}}_j = \mathbf{X}_j^\dagger \mathbf{\tilde Y}_j$, we have
\begin{equation}
\label{eq:Theorem1_1}
  {\mathbf{W}}= \begin{bmatrix} \mathcal{W}_i\mathbf{W}_i + \mathcal{W}_j\mathbf{\hat W}_j & \mathcal{W}_j\mathbf{\check W}_j \end{bmatrix},
\end{equation}
where
\begin{equation}
\label{eq:Theorem1_2}
  \begin{cases}
\mathcal{W}_i = \mathbf{I} - \mathbf{M}_i^{-1} \mathbf{M}_j - \mathbf{M}_i^{-1} \mathbf{M}_j (\mathbf{M}_i + \mathbf{M}_j)^{-1} \mathbf{M}_j, \\
\mathcal{W}_j = \mathbf{I} - \mathbf{M}_j^{-1} \mathbf{M}_i - \mathbf{M}_j^{-1} \mathbf{M}_i (\mathbf{M}_i + \mathbf{M}_j)^{-1} \mathbf{M}_i, \\
\mathbf{M}_i = \mathbf{X}_i^\top \mathbf{X}_i, \quad \quad \mathbf{M}_j = \mathbf{X}_j^\top \mathbf{X}_j.
\end{cases}
\end{equation}


\noindent \textit{Proof.} Firstly, according to Lemma 1, it is established that:
\begin{equation}
\label{eq:appendix2_1}
  \mathbf{X}^{\dagger}=\begin{bmatrix}\bar{\mathbf{U}}&\bar{\mathbf{V}}\end{bmatrix},
\end{equation}
where
\begin{equation}
\label{eq:appendix2_2}
\begin{cases}
\mathbf{\bar{U}} = \left[\mathbf{I} - \mathbf{R}_i \mathbf{M}_j - \mathbf{R}_i \mathbf{M}_j (\mathbf{M}_i + \mathbf{M}_j)^{-1} \mathbf{M}_j \right] \mathbf{X}_i^\dagger \\
\mathbf{\bar{V}} = \left[\mathbf{I} - \mathbf{R}_j \mathbf{M}_i - \mathbf{R}_j \mathbf{M}_i (\mathbf{M}_i + \mathbf{M}_j)^{-1} \mathbf{M}_i \right] \mathbf{X}_j^\dagger
\end{cases},
\begin{cases}
\mathbf{M}_i = \mathbf{X}_i^\top \mathbf{X}_i \\
\mathbf{M}_j = \mathbf{X}_j^\top \mathbf{X}_j
\end{cases},
\begin{cases}
\mathbf{R}_i = \mathbf{M}_i^{-1} \\
\mathbf{R}_j = \mathbf{M}_j^{-1}
\end{cases}.
\end{equation}

\noindent Consequently, $\mathbf{W}$ can be computed as follows:
\begin{equation}
\label{eq:appendix2_3}
  \mathbf{W} = \mathbf{X}^{\dagger} \mathbf{Y} = \begin{bmatrix} \mathbf{\bar{U}} & \mathbf{\bar{V}} \end{bmatrix} \begin{bmatrix} \mathbf{Y}_i & \textbf{0} \\ \mathbf{\bar Y}_j & \mathbf{\tilde Y}_j  \end{bmatrix} = \begin{bmatrix} \mathbf{\bar{U}}\mathbf{Y}_i + \mathbf{\bar{V}}\mathbf{\bar Y}_j & \mathbf{\bar{V}} \mathbf{\tilde Y}_j \end{bmatrix}.
\end{equation}

\noindent By substituting (\ref{eq:appendix2_2}) into (\ref{eq:appendix2_3}), we obtain
\begin{equation}
\label{eq:appendix2_4}
\begin{aligned}
  \mathbf{W} =  \lbrack \left(\mathbf{I} - \mathbf{R}_i \mathbf{M}_j - \mathbf{R}_i \mathbf{M}_j (\mathbf{M}_i + \mathbf{M}_j)^{-1} \mathbf{M}_j \right) \mathbf{X}_i^\dagger \mathbf{Y}_i + \left(\mathbf{I}-\mathbf{R}_j\mathbf{M}_i-\mathbf{R}_j\mathbf{M}_i(\mathbf{M}_i+\mathbf{M}_j)^{-1}\mathbf{M}_i\right)\mathbf{X}_j^\dagger \mathbf{\bar Y}_j \\
  \left(\mathbf{I}-\mathbf{R}_j\mathbf{M}_i-\mathbf{R}_j\mathbf{M}_i(\mathbf{M}_i+\mathbf{M}_j)^{-1}\mathbf{M}_i\right)\mathbf{X}_j^\dagger \mathbf{\tilde Y}_j\rbrack.
\end{aligned}
\end{equation}

\noindent That is,
\begin{equation}
\label{eq:appendix2_5}
  \mathbf{W}= \begin{bmatrix} \mathcal{W}_i\mathbf{W}_i + \mathcal{W}_j\mathbf{\hat W}_j & \mathcal{W}_j\mathbf{\check W}_j \end{bmatrix},
\end{equation}
where
\begin{equation}
\label{eq:appendix2_6}
  \begin{cases}
\mathcal{W}_i = \mathbf{I} - \mathbf{R}_i \mathbf{M}_j - \mathbf{R}_i \mathbf{M}_j (\mathbf{M}_i + \mathbf{M}_j)^{-1} \mathbf{M}_j\\
\mathcal{W}_j = \mathbf{I} - \mathbf{R}_j \mathbf{M}_i - \mathbf{R}_j \mathbf{M}_i (\mathbf{M}_i + \mathbf{M}_j)^{-1} \mathbf{M}_i
\end{cases}
\begin{cases}
\mathbf{M}_i = \mathbf{X}_i^\top \mathbf{X}_i\\
\mathbf{M}_j = \mathbf{X}_j^\top \mathbf{X}_j
\end{cases}
\begin{cases}
\mathbf{R}_i = \mathbf{M}_i^{-1}\\
\mathbf{R}_j = \mathbf{M}_j^{-1}
\end{cases}.
\end{equation}

\hfill $\blacksquare$




\noindent \textbf{Theorem 1.} Let $\mathbf{X}_{1:k} = \begin{bmatrix} \mathbf{X}_{1:k-1} \\ \mathbf{X}_k\end{bmatrix}$ and $\mathbf{Y}_{1:k} = \begin{bmatrix} \mathbf{Y}_{1:k-1} & \textbf{0} \\ \mathbf{\bar Y}_{k} & \mathbf{\tilde Y}_{k}  \end{bmatrix}$ represent the feature matrix and label matrix of the first $k$ clients' complete dataset, where $\mathbf{X}_{1:k-1}$ and $\mathbf{X}_k$ both have full column ranks. Meanwhile, we denote $\mathbf{W}_{\mathrm{agg},k}$ as the optimal weights of the global model, i.e., $\mathbf{W}_{\mathrm{agg},k} = \mathbf{X}_{1:k}^\dagger \mathbf{Y}_{1:k}$, we have
\begin{equation}
\label{eq:Theorem1_1}
  {\mathbf{W}_{\mathrm{agg},k}}= \begin{bmatrix} \mathcal{W}_{\mathrm{agg},k-1} \mathbf{W}_{\mathrm{agg},k-1} + \mathcal{W}_k\mathbf{\hat W}_k & \mathcal{W}_k\mathbf{\check W}_k \end{bmatrix},
\end{equation}
where
\begin{equation}
\label{eq:Theorem1_2}
  \begin{cases}
\mathcal{W}_{\mathrm{agg},k} = \mathbf{I} - (\mathbf{M}_{\mathrm{agg}, k-1})^{-1} \mathbf{M}_k (\mathbf{I} + (\mathbf{M}_{\mathrm{agg}, k})^{-1} \mathbf{M}_k), \\
\mathcal{W}_k = \mathbf{I} - \mathbf{M}_k^{-1} \mathbf{M}_{\mathrm{agg}, k-1} (\mathbf{I} + \mathbf{M}_{\mathrm{agg}, k}^{-1} \mathbf{M}_{\mathrm{agg}, k-1}), \\
\mathbf{M}_{\mathrm{agg}, k} = \sum_i^k \mathbf{M}_i, \quad \mathbf{M}_i = \mathbf{X}_i^\top \mathbf{X}_i.
\end{cases}
\end{equation}

\noindent \textit{Proof.}
Building upon the \textbf{Proposition 3}, we can further extend the model aggregation from two clients to multiple clients.
when the $k$-th client connects to the server, the server's global model is denoted as $\mathbf{W}_{\mathrm{agg},k-1}$ and the client's local model as $\mathbf{\hat W}_k, \mathbf{\check W}_k$. 
Following aggregation, the global model $\mathbf{W}_{\mathrm{agg},k}$ can be computed as follows:

\begin{equation}
\label{eq:aggregation_1}
\mathbf{W}_{\mathrm{agg},k} = \begin{bmatrix} \mathbf{\mathcal{W}}_{\mathrm{agg},k}\mathbf{W}_{\mathrm{agg},k-1} + \mathcal{W}_k\mathbf{\hat W}_k & \mathcal{W}_k\mathbf{\check W}_k \end{bmatrix},
\end{equation}

\noindent By substituting $\mathbf{M}_{\mathrm{agg},k-1}$, $\mathbf{M}_{k}$ for $\mathbf{M}_u$, $\mathbf{M}_v$ in (\ref{eq:Theorem1_2}), we can obtain:
\begin{equation}
  \mathbf{M}_{\mathrm{agg},k} = \mathbf{M}_{\mathrm{agg},k-1} + \mathbf{M}_k = \sum_i^k \mathbf{M}_{k}.
\end{equation}


\noindent Hence,
% \begin{equation}
% \label{eq:aggregation_2}
%   \begin{cases}
% \mathcal{W}_{\mathrm{agg},k} = \mathbf{I} - (\mathbf{M}_{\mathrm{agg}, k-1})^{-1} \mathbf{M}_k (\mathbf{I} + (\mathbf{M}_{\mathrm{agg}, k})^{-1} \mathbf{M}_k), \\
% \mathcal{W}_k = \mathbf{I} - \mathbf{M}_k^{-1} \mathbf{M}_{\mathrm{agg}, k-1} (\mathbf{I} + \mathbf{M}_{\mathrm{agg}, k}^{-1} \mathbf{M}_{\mathrm{agg}, k-1}), \\
% \mathbf{M}_{\mathrm{agg}, k} = \sum_i^k \mathbf{M}_i, \quad \mathbf{M}_i = \mathbf{X}_i^\top \mathbf{X}_i.
% \end{cases}
% \end{equation}
\begin{equation}
\begin{aligned}
    \mathcal{W}_{\mathrm{agg},k} &= \mathbf{I} - (\mathbf{M}_{\mathrm{agg}, k-1})^{-1} \mathbf{M}_k (\mathbf{I} + (\mathbf{M}_{\mathrm{agg}, k-1} + \mathbf{M}_{k})^{-1} \mathbf{M}_k) \\
    &= \mathbf{I} - (\mathbf{M}_{\mathrm{agg}, k-1})^{-1} \mathbf{M}_k (\mathbf{I} + (\mathbf{M}_{\mathrm{agg}, k})^{-1} \mathbf{M}_k),
\end{aligned}
\end{equation}
\begin{equation}
\begin{aligned}
    \mathcal{W}_k &= \mathbf{I} - \mathbf{M}_k^{-1} \mathbf{M}_{\mathrm{agg}, k-1} (\mathbf{I} + (\mathbf{M}_{\mathrm{agg}, k-1} + \mathbf{M}_{k})^{-1} \mathbf{M}_{\mathrm{agg}, k-1}) \\
    &= \mathbf{I} - \mathbf{M}_k^{-1} \mathbf{M}_{\mathrm{agg}, k-1} (\mathbf{I} + \mathbf{M}_{\mathrm{agg}, k}^{-1} \mathbf{M}_{\mathrm{agg}, k-1}).
\end{aligned}
\end{equation}


\hfill $\blacksquare$











\noindent \textbf{Proposition 4.} Let $\mathbf{W}$ and $\mathbf{W}^\mathrm{r}$ represent the outcomes of \eqref{eq:Theorem1-1} and \eqref{eq:server-3} with the dataset $\mathbf{X} = \begin{bmatrix} \mathbf{X}_i \\ \mathbf{X}_j\end{bmatrix}$ and $\mathbf{Y} = \begin{bmatrix} \mathbf{Y}_i & \textbf{0} \\ \mathbf{\bar Y}_j & \mathbf{\tilde Y}_j  \end{bmatrix}$, their relationship can be established as follows:
\begin{equation}
\label{eq:Proposition4-1}
\mathbf{W}=(\mathbf{M}_i^{\mathrm{r}} + \mathbf{M}_j^{\mathrm{r}} - 2 \gamma \mathbf{I})^{-1} (\mathbf{M}_i^{\mathrm{r}} + \mathbf{M}_j^{\mathrm{r}}) \mathbf{W}^{\mathrm{r}},
\end{equation}
where
\begin{equation}
\label{eq:Proposition4-2}
  \mathbf{M}_i^\mathrm{r} = \mathbf{X}_i^\top \mathbf{X}_i + \gamma \mathbf{I}, \quad \mathbf{M}_j^\mathrm{r} = \mathbf{X}_j^\top \mathbf{X}_j + \gamma \mathbf{I}.
\end{equation}

\noindent \textit{Proof.} Initially, based on \eqref{eq:server-3}, we can obtain:
\begin{equation}
\mathbf{W}^\mathrm{r} = \begin{bmatrix} \mathbf{\mathcal{W}}_i^\mathrm{r}  \mathbf{W}_i^\mathrm{r} + \mathcal{W}_j^\mathrm{r}  \mathbf{\hat W}_j^\mathrm{r} & \mathcal{W}_j^\mathrm{r}  \mathbf{\check W}_j^\mathrm{r} \end{bmatrix},
\end{equation}
where
\begin{equation}
\begin{cases}
\mathcal{W}_i^\mathrm{r} = \mathbf{I} - (\mathbf{M}_i^\mathrm{r})^{-1} \mathbf{M}_j^\mathrm{r} (\mathbf{I} + (\mathbf{M}_i^\mathrm{r} + \mathbf{M}_j^\mathrm{r})^{-1} \mathbf{M}_j),  \\
\mathcal{W}_j^\mathrm{r}  = \mathbf{I} - (\mathbf{M}_j^\mathrm{r})^{-1} \mathbf{M}_i^\mathrm{r} (\mathbf{I} + (\mathbf{M}_i^\mathrm{r} + \mathbf{M}_j^\mathrm{r})^{-1} \mathbf{M}_i^\mathrm{r}), \\
\mathbf{M}_i^\mathrm{r} = \mathbf{X}_i^\top \mathbf{X}_i +\gamma\mathbf{I}, \quad
\mathbf{M}_j^\mathrm{r} = \mathbf{X}_j^\top \mathbf{X}_j +\gamma\mathbf{I}.
\end{cases}
\end{equation}

\noindent Following this, given that $\mathbf{W}_i^\mathrm{r} = (\mathbf{X}_i^\top \mathbf{X}_i + \gamma \mathbf{I})^{-1} \mathbf{X}_i^\top \mathbf{Y}_i$ then
\begin{equation}
\label{eq:appendix3_3}
  \begin{aligned}
\mathcal{W}_{i}^{\mathrm{r}}\mathbf{{W}}_{i}^{\mathrm{r}} &= [\mathbf{I} - (\mathbf{M}_i^\mathrm{r})^{-1} \mathbf{M}_j^\mathrm{r} (\mathbf{I} + (\mathbf{M}_i^\mathrm{r} + \mathbf{M}_j^\mathrm{r})^{-1} \mathbf{M}_j^\mathrm{r})] (\mathbf{X}_i^\top \mathbf{X}_i + \gamma \mathbf{I})^{-1} \mathbf{X}_i^\top \mathbf{Y}_i \\
&= [\mathbf{I} - (\mathbf{M}_i^\mathrm{r})^{-1} \mathbf{M}_j^\mathrm{r} (\mathbf{I} + (\mathbf{M}_i^\mathrm{r} + \mathbf{M}_j^\mathrm{r})^{-1} \mathbf{M}_j^\mathrm{r})] (\mathbf{M}_i^\mathrm{r})^{-1} \mathbf{X}_i^\top \mathbf{Y}_i \\
&= [(\mathbf{M}_i^\mathrm{r})^{-1} - (\mathbf{M}_i^\mathrm{r})^{-1} \mathbf{M}_j^\mathrm{r} (\mathbf{I} + (\mathbf{M}_i^\mathrm{r} + \mathbf{M}_j^\mathrm{r})^{-1} \mathbf{M}_j^\mathrm{r})(\mathbf{M}_i^\mathrm{r})^{-1}] \mathbf{X}_i^\top \mathbf{Y}_i \\
&= [(\mathbf{M}_i^\mathrm{r})^{-1} - (\mathbf{M}_i^\mathrm{r})^{-1} \mathbf{M}_j^\mathrm{r} (\mathbf{M}_i^\mathrm{r})^{-1} - (\mathbf{M}_i^\mathrm{r})^{-1} \mathbf{M}_j^\mathrm{r} (\mathbf{M}_i^\mathrm{r} + \mathbf{M}_j^\mathrm{r})^{-1} \mathbf{M}_j^\mathrm{r} (\mathbf{M}_i^\mathrm{r})^{-1}] \mathbf{X}_i^\top \mathbf{Y}_i .
% [\mathbf{I}-\mathbf{R}_i^\mathrm{r}\mathbf{M}_j^\mathrm{r}-\mathbf{R}_i^\mathrm{r}\mathbf{M}_j^\mathrm{r}(\mathbf{M}_i^\mathrm{r}+\mathbf{M}_j^\mathrm{r})^{-1}\mathbf{M}_j^\mathrm{r}]\mathbf{R}_i^\mathrm{r}\mathbf{X}_i^\top\mathbf{Y}_i\\
% &=[\mathbf{R}_i^\mathrm{r}-\mathbf{R}_i^\mathrm{r}\mathbf{M}_j^\mathrm{r}\mathbf{R}_i^\mathrm{r}-\mathbf{R}_i^\mathrm{r}\mathbf{M}_j^\mathrm{r}(\mathbf{M}_i^\mathrm{r}+\mathbf{M}_j^\mathrm{r})^{-1}\mathbf{M}_j^\mathrm{r}\mathbf{R}_i^\mathrm{r}]\mathbf{X}_i^\top\mathbf{Y}_i.
\end{aligned}
\end{equation}

\noindent Subsequently, based on the Woodbury Matrix Identity as presented in (\ref{eq:appendix1_9}), we substitute both $\mathbf{B}$ and $\mathbf{D}$ with $\mathbf{I}$. This adjustment allows us to derive:
\begin{equation}
\label{eq:appendix3_4}
(\mathbf{A}+\mathbf{E})^{-1}=\mathbf{A}^{-1}-\mathbf{A}^{-1}(\mathbf{A}^{-1}+\mathbf{E}^{-1})^{-1}\mathbf{A}^{-1}
\end{equation}

\noindent Further, it can be obtained:
\begin{equation}
\label{eq:appendix3_5}
\mathbf{A}^{-1}(\mathbf{A}^{-1}+\mathbf{E}^{-1})^{-1}\mathbf{A}^{-1} = \mathbf{A}^{-1} - (\mathbf{A}+\mathbf{E})^{-1}.
\end{equation}

\noindent Subsequently, replacing $\mathbf{A}^{-1}$ and $\mathbf{E}^{-1}$ in (\ref{eq:appendix3_5}) with $\mathbf{M}_i^\mathrm{r}$ and $\mathbf{M}_j^\mathrm{r}$ respectively, yields:
\begin{equation}
\label{eq:appendix3_6}
\mathbf{M}_j^\mathrm{r}(\mathbf{M}_j^\mathrm{r}+\mathbf{M}_i^\mathrm{r})^{-1}\mathbf{M}_j^\mathrm{r} = \mathbf{M}_j^\mathrm{r} - ( (\mathbf{M}_i^\mathrm{r})^{-1} + (\mathbf{M}_j^\mathrm{r})^{-1} )^{-1}
\end{equation}

\noindent Similarly,
\begin{equation}
\label{eq:appendix3_7}
(\mathbf{M}_i^\mathrm{r})^{-1} ( (\mathbf{M}_i^\mathrm{r})^{-1} + (\mathbf{M}_j^\mathrm{r})^{-1} )^{-1} (\mathbf{M}_i^\mathrm{r})^{-1} = (\mathbf{M}_i^\mathrm{r})^{-1} - (\mathbf{M}_i^\mathrm{r}+\mathbf{M}_j^\mathrm{r})^{-1}
\end{equation}

\noindent Initially, incorporating (\ref{eq:appendix3_6}) into (\ref{eq:appendix3_3}), we find:
\begin{equation}
\label{eq:appendix3_8}
\begin{aligned}
\mathbf{\mathcal{W}}_i^\mathrm{r}\mathbf{\hat{W}}_i^\mathrm{r} &= [(\mathbf{M}_i^\mathrm{r})^{-1} - (\mathbf{M}_i^\mathrm{r})^{-1} \mathbf{M}_j^\mathrm{r} (\mathbf{M}_i^\mathrm{r})^{-1} - (\mathbf{M}_i^\mathrm{r})^{-1} \mathbf{M}_j^\mathrm{r} (\mathbf{M}_i^\mathrm{r} + \mathbf{M}_j^\mathrm{r})^{-1} \mathbf{M}_j^\mathrm{r} (\mathbf{M}_i^\mathrm{r})^{-1}] \mathbf{X}_i^\top \mathbf{Y}_i \\
&= [(\mathbf{M}_i^\mathrm{r})^{-1} - (\mathbf{M}_i^\mathrm{r})^{-1} \mathbf{M}_j^\mathrm{r} (\mathbf{M}_i^\mathrm{r})^{-1} + (\mathbf{M}_i^\mathrm{r})^{-1} \mathbf{M}_j^\mathrm{r} (\mathbf{M}_i^\mathrm{r})^{-1} - (\mathbf{M}_i^\mathrm{r})^{-1} ( (\mathbf{M}_i^\mathrm{r})^{-1} + (\mathbf{M}_j^\mathrm{r})^{-1} )^{-1} (\mathbf{M}_i^\mathrm{r})^{-1}] \mathbf{X}_i^\top \mathbf{Y}_i \\
&= [(\mathbf{M}_i^\mathrm{r})^{-1} - (\mathbf{M}_i^\mathrm{r})^{-1} ( (\mathbf{M}_i^\mathrm{r})^{-1} + (\mathbf{M}_j^\mathrm{r})^{-1} )^{-1} (\mathbf{M}_i^\mathrm{r})^{-1}] \mathbf{X}_i^\top \mathbf{Y}_i
\end{aligned}
\end{equation}


\noindent Proceeding to integrate (\ref{eq:appendix3_5}) into (\ref{eq:appendix3_8}), we can determine:
\begin{equation}
\label{eq:appendix3_9}
\begin{aligned}
\mathbf{\mathcal{W}}_i^\mathrm{r} \mathbf{W}_i^\mathrm{r} 
&= [(\mathbf{M}_i^\mathrm{r})^{-1} - (\mathbf{M}_i^\mathrm{r})^{-1} ( (\mathbf{M}_i^\mathrm{r})^{-1} + (\mathbf{M}_j^\mathrm{r})^{-1} )^{-1} (\mathbf{M}_i^\mathrm{r})^{-1}] \mathbf{X}_i^\top \mathbf{Y}_i \\
&= [(\mathbf{M}_i^\mathrm{r})^{-1} - (\mathbf{M}_i^\mathrm{r})^{-1} + (\mathbf{M}_i^\mathrm{r}+\mathbf{M}_j^\mathrm{r})^{-1}] \mathbf{X}_i^\top \mathbf{Y}_i \\
&= (\mathbf{M}_i^\mathrm{r}+\mathbf{M}_j^\mathrm{r})^{-1} \mathbf{X}_i^\top \mathbf{Y}_i.
\end{aligned}
\end{equation}

\noindent Similarly, we can obtain:
\begin{equation}
\label{eq:appendix3_10}
\mathbf{\mathcal{W}}_j^\mathrm{r} \mathbf{\hat{W}}_j^\mathrm{r} = (\mathbf{M}_i^\mathrm{r}+\mathbf{M}_j^\mathrm{r})^{-1} \mathbf{X}_j^\top \mathbf{\bar Y}_j.
\end{equation}

\begin{equation}
\label{eq:appendix3_10}
\mathbf{\mathcal{W}}_j^\mathrm{r} \mathbf{\check{W}}_j^\mathrm{r} = (\mathbf{M}_i^\mathrm{r}+\mathbf{M}_j^\mathrm{r})^{-1} \mathbf{X}_j^\top \mathbf{\tilde Y}_j.
\end{equation}

\noindent Combining (\ref{eq:appendix3_9}), (\ref{eq:appendix3_10}), and (\ref{eq:appendix3_1}) can be expressed as:
\begin{equation}
\label{eq:appendix3_11}
\begin{aligned}
\mathbf{W}^\mathrm{r} 
& = \begin{bmatrix} \mathbf{\mathcal{W}}_i^\mathrm{r}  \mathbf{W}_i^\mathrm{r} + \mathcal{W}_j^\mathrm{r}  \mathbf{\hat W}_j^\mathrm{r} & \mathcal{W}_j^\mathrm{r}  \mathbf{\check W}_j^\mathrm{r} \end{bmatrix}
 \\
& = (\mathbf{M}_i^\mathrm{r}+\mathbf{M}_j^\mathrm{r})^{-1} \begin{bmatrix} \mathbf{X}_i^\top \mathbf{Y}_i + \mathbf{X}_j^\top \mathbf{\bar Y}_j & \mathbf{X}_j^\top \mathbf{\tilde Y}_j\end{bmatrix}.
\end{aligned}
\end{equation}

\noindent Given that ${\mathbf{W}} = \mathbf{X}^\dagger \mathbf{Y}$, where $\mathbf{X} = \begin{bmatrix} \mathbf{X}_i \\ \mathbf{X}_j \end{bmatrix}$ and $\mathbf{Y} = \begin{bmatrix} \mathbf{Y}_i & \textbf{0} \\ \mathbf{\bar Y}_j & \mathbf{\tilde Y}_j \end{bmatrix}$, ${\mathbf{W}}$ can be calculated as:
\begin{equation}
\label{eq:appendix3_12}
\begin{aligned}
\mathbf{W}& =\mathbf{X}^\dagger\mathbf{Y}\\
&=(\mathbf{X}^\mathrm{T}\mathbf{X})^{-1}\mathbf{X}^\mathrm{T}\mathbf{Y} \\
&=(\begin{bmatrix}\mathbf{X}_i^\mathrm{T}&\mathbf{X}_j^\mathrm{T}\end{bmatrix}\begin{bmatrix}\mathbf{X}_i\\\mathbf{X}_j\end{bmatrix})^{-1}\begin{bmatrix}\mathbf{X}_i^\mathrm{T}&\mathbf{X}_j^\mathrm{T}\end{bmatrix}\begin{bmatrix} \mathbf{Y}_i & \textbf{0} \\ \mathbf{\bar Y}_j & \mathbf{\tilde Y}_j \end{bmatrix} \\
&=(\mathbf{X}_i^\top\mathbf{X}_i+\mathbf{X}_j^\top\mathbf{X}_j)^{-1}\begin{bmatrix} \mathbf{X}_i^\top\mathbf{Y}_i + \mathbf{X}_j^\top\mathbf{\bar Y}_j & \mathbf{X}_j^\top\mathbf{\tilde Y}_j\end{bmatrix} \\
&=(\mathbf{M}_i^\mathrm{r}+\mathbf{M}_j^\mathrm{r} - 2 \gamma \mathbf{I})^{-1}\begin{bmatrix} \mathbf{X}_i^\top\mathbf{Y}_i + \mathbf{X}_j^\top\mathbf{\bar Y}_j & \mathbf{X}_j^\top\mathbf{\tilde Y}_j\end{bmatrix}.
\end{aligned}
\end{equation}


\noindent Observing (\ref{eq:appendix3_11}) and (\ref{eq:appendix3_12}) reveals the following relationship between:
\begin{equation}
\begin{aligned}
    &(\mathbf{M}_i^\mathrm{r}+\mathbf{M}_j^\mathrm{r} - 2 \gamma \mathbf{I}) \mathbf{W} = (\mathbf{M}_i^\mathrm{r}+\mathbf{M}_j^\mathrm{r}) \mathbf{W}^\mathrm{r} \\
    \Rightarrow & \mathbf{W} = (\mathbf{M}_i^\mathrm{r}+\mathbf{M}_j^\mathrm{r} - 2 \gamma \mathbf{I})^{-1} (\mathbf{M}_i^\mathrm{r}+\mathbf{M}_j^\mathrm{r}) \mathbf{W}^\mathrm{r}.
\end{aligned}
\end{equation}

\hfill $\blacksquare$








\noindent \textbf{Theorem 2.} Let $\mathbf{W}_{\mathrm{agg},k}$ and $\mathbf{W}_{\mathrm{agg},k}^\mathrm{r}$ represent the outcomes of \eqref{eq:Theorem1-1} and \eqref{eq:server-3} with the dataset $\{ \mathbf{X}_{1:k} , \mathbf{Y}_{1:k} \}$, their relationship can be established as follows:
\begin{equation}
\label{eq:Theorem2_1}
    \mathbf{W}_{\mathrm{agg},k} = (\mathbf{M}_{\mathrm{agg},k}^{\mathrm{r}} - k\gamma \mathbf{I})^{-1} \mathbf{M}_{\mathrm{agg},k}^{\mathrm{r}} \mathbf{W}_{\mathrm{agg},k}^{\mathrm{r}},
\end{equation}
where
\begin{equation}
\label{eq:Theorem2_2}
  \mathbf{M}_{\mathrm{agg},k}^\mathrm{r} = \sum_{i=1}^k \mathbf{M}_i^\mathrm{r}, \quad \mathbf{M}_i^\mathrm{r} = \mathbf{X}_i^\top \mathbf{X}_i + \gamma \mathbf{I}.
\end{equation}


\noindent \textit{Proof.}
Building upon the \textbf{Proposition 4}, we can further extend the model aggregation from two clients to multiple clients.
Specifically, we employ $\mathbf{W}_{\mathrm{agg},k-1}^\mathrm{r}$, $\mathbf{W}_{\mathrm{agg},k-1}$, $\mathbf{M}_{\mathrm{agg},k-1}^{\mathrm{r}}$, and $\mathbf{M}_k^\mathrm{r}$ to substitute for $\mathbf{W}^\mathrm{r}$, $\mathbf{W}$, $\mathbf{M}_{i}^{\mathrm{r}}$, and $\mathbf{M}_j^\mathrm{r}$ in  (\ref{eq:Proposition4-1}) and (\ref{eq:Proposition4-2}), i.e.
\begin{equation}
\label{eq:Theorem2_1}
    \mathbf{W}_{\mathrm{agg},k} = (\mathbf{M}_{\mathrm{agg},k-1}^{\mathrm{r}} + \mathbf{M}_{k}^{\mathrm{r}} - k \gamma \mathbf{I})^{-1} (\mathbf{M}_{\mathrm{agg},k-1}^{\mathrm{r}} + \mathbf{M}_{k}^{\mathrm{r}}) \mathbf{W}_{\mathrm{agg},k}^{\mathrm{r}}.
\end{equation}

\noindent Since 
\begin{equation}
\label{eq:Theorem2_2}
  \mathbf{M}_{\mathrm{agg},k}^\mathrm{r} = \sum_{i=1}^k \mathbf{M}_i^\mathrm{r}, \quad \mathbf{M}_i^\mathrm{r} = \mathbf{X}_i^\top \mathbf{X}_i + \gamma \mathbf{I},
\end{equation}
we can obtain:
\begin{equation}
\label{eq:Theorem2_1}
\begin{aligned}
    \mathbf{W}_{\mathrm{agg},k} &= (\mathbf{M}_{\mathrm{agg},k-1}^{\mathrm{r}} + \mathbf{M}_{k}^{\mathrm{r}} - k \gamma \mathbf{I})^{-1} (\mathbf{M}_{\mathrm{agg},k-1}^{\mathrm{r}} + \mathbf{M}_{k}^{\mathrm{r}}) \mathbf{W}_{\mathrm{agg},k}^{\mathrm{r}} \\
    &=(\mathbf{M}_{\mathrm{agg},k}^{\mathrm{r}} - k\gamma \mathbf{I})^{-1} \mathbf{M}_{\mathrm{agg},k}^{\mathrm{r}} \mathbf{W}_{\mathrm{agg},k}^{\mathrm{r}}.
\end{aligned}
\end{equation}

\hfill $\blacksquare$
